# Supplementary material for: A Cohesive Distillation Architecture for Neural Language Models
Source: arXiv:2301.08130 source file (2023-01-29)
Supplement: Supplementary file 1 [file AppendixTemplate.tex]

% Appendix Template

\chapter{Appendix Title Here} \label{AppendixX}

Write your Appendix content here.
